# Supplementary material for: EditShield: Protecting Unauthorized Image Editing by Instruction-guided Diffusion Models
Source: arXiv:2311.12066 source file (2024-07-17)
Supplement: Supplementary file 1 [file appendix-camera-ready.tex]

\title{Appendix\\ \texttt{EditShield}: Protecting Unauthorized Image Editing by Instruction-guided Diffusion Models}

\titlerunning{EditShield}
\author{
  Ruoxi Chen\inst{1}\orcidlink{0000-0003-2626-5448} \and 
  Haibo Jin\inst{2}\orcidlink{0000-0002-7244-7659} \and 
  Yixin Liu\inst{3}\orcidlink{0000-0003-3856-439X} \and
  Jinyin Chen\inst{1}\thanks{Corresponding author} \and 
  Haohan Wang\inst{2}\orcidlink{0000-0002-1826-4069} \and 
  Lichao Sun\inst{3}
}

% TODO FINAL: Replace with an abbreviated list of authors.
\authorrunning{R.~Chen et al.}
% First names are abbreviated in the running head.
% If there are more than two authors, 'et al.' is used.

% TODO FINAL: Replace with your institution list.
\institute{
  Zhejiang University of Technology, Hangzhou, China\\
\email{\{2112003149,chenjinyin\}@zjut.edu.cn}\\ \and
  University of Illinois Urbana-Champaign, Champaign, USA\\
  \email{\{haibo,haohanw\}@illinois.edu}
  \and
  Lehigh University, Bethlehem, USA\\
  \email{\{yila22,lis221\}@lehigh.edu}
}

\maketitle

In this supplementary document, we first present the pseudo-code in Section~\ref{alg}. We then describe experimental details in Section~\ref{details}.
We further provide more experimental results in Section \ref{more_res}. 
% describe more details on XXX and more implementation details
% in Sec. XXX, and discuss our limitation in Sec. D. Finally, we show more qualitative
% results in Sec. E. 

\section{\method Algorithm \label{alg}}
\method works by introducing strategic perturbations that effectively disrupt the latent representations of the instruction-guided diffusion model. The pseudo-code of \method is presented in Algorithm~\ref{algo}. 

% EditShield is available online as a plug-and-play toolkit~\footnote{https://anonymous.4open.science/status/0FDD}.
 
\begin{algorithm}[htbp]
\caption{\method}
\begin{algorithmic}[1]
\Require A set of input images $D = \{x_1, x_2, \dots, x_N\}$,  VAE $\mathcal{E}$ in instruction-guided diffusion model, step size $\alpha$, overall perturbation budget $\xi$, maximum iterations $S$, hyper-parameter $\beta$, a set of transformations $T$
% \Statex Intermediate layer function $f_{l}(\cdot)$
% \Statex $\ell_2$ distance threshold $\tau$
% \Ensure Universal protection perturbation $\delta^*$
% \Statex Shield perturbation $\left \| \delta  \right \| _{p} \le \xi $
\State Initialize perturbation $\delta \leftarrow Gaussian~noise \mathcal~{N}(0, \mathbf{I}$)
% \State Initialize $\ell_2$ distance measure $Dist(\cdot,\cdot)$
% \For{$t = 1$ \textbf{to} $S$}
    \For{each $x_i$ in $D$}
        \State $x'_i \leftarrow x_i + \delta $
        \State Calculate the embedding $z_i=\mathcal{E}(x_i)$
        \State Calculate the protected embedding $z'_i=\mathcal{E}(x'_i)$
       % %\State Calculate the $Dist(z_i,z'_i)$ 
        % \State $e_i \leftarrow f_{l}(x_i)$, $e'_i \leftarrow f_{l}(x'_i)$
        %\If{$Dist(z_i,z'_i) < \tau$}
        \State Sampling a transformation function $t, t \in T$
        \State $g \leftarrow \nabla_{x_p}  \mathbb{E}_{t\sim T} [Dist((\mathcal{E}(t(x_p)),\mathcal{E}(x))]- \beta \cdot ||x_p-x||_{2}^{2}$
            
        % \State $g \leftarrow \nabla_x Dist(z_i,z'_i)$ 
        % \State \textit{s.t.} $\mathop{\arg\max} Dist(z_i,z'_i)$
        \State $r_i \leftarrow \frac{g}{\|g\|_2}$
        \State Update perturbation $\delta  \leftarrow \delta  + \alpha \cdot r_i$
        \State $\delta = clip(\delta, -\xi, \xi)$ 
        % \State $\delta \leftarrow \min\left(\xi, \|\delta\|_2\right) \cdot \frac{\delta}{\|\delta\|_2}$
        %\EndIf
    \EndFor
% \EndFor
\State \Return Protected image $x_{i,p}=x_i+\delta$
\end{algorithmic}
\label{algo}
\end{algorithm}

\section{Experimental Details\label{details}}
\subsection{Details of image editing models}
For image editing, we use the open-source instruction-guided diffusion models InstructPix2Pix (ip2p) and its fine-tuned version on MagicBrush (ip2p-mb), whose checkpoints from GitHub~\footnote{https://github.com/timothybrooks/instruct-pix2pix/} and Hugging Face~\footnote{https://huggingface.co/osunlp/InstructPix2Pix-MagicBrush/}, respectively. 
To mitigate randomness, we use the same seed when editing source and protected images. 

The default configurations for both models are: The number of steps is set to 100, image\_guidance\_scale=1.2 and text\_guidance\_scale=7.5. The image size is 512 $\times$ 512.

\subsection{Computational cost}
All experiments are conducted on one NVIDIA GeForce RTX 4090 24GB GPU. On ip2p model, EditShield requires 8560 MiB of memory to generate protection.

EditShield does not require training of the model. The time complexity of it is $\mathcal{O}(n)$, where $n$ is the number of images to be protected. In practice, it takes 2.46s on average to generate the protection per image.

\subsection{Query models and prompts}
Some models are adopted to help us for evaluations. We will detail prompts that we use and then give some examples. In general, links of those models are shown in Table~\ref{links}.

\begin{table}[htbp]
    \centering
    
    \caption{Links to query models.}
    \resizebox{0.8\linewidth}{!}{
    \begin{tabular}{ll}
\hline
\textbf{Model} & \textbf{Model links}                                  \\ \hline
LLaVA-1.5 13B & \url{https://huggingface.co/liuhaotian/llava-v1.5-13b} \\
GPT-4V         & \url{https://chat.openai.com/} \\
GPT-3.5-Turbo  &  \url{https://chat.openai.com/} \\ \hline
\end{tabular}}
\vspace{-10pt}
\label{links}
\vspace{-10pt}
\end{table}

\subsubsection{Generate text descriptions}
We adopt LLaVA-1.5 13B for generating text descriptions of both the source and edited images without and with protection. The implementation of the input template follows the chatbot template of LLaMA-2-13B-Chat. Specifically, the following input template is applied for LLaVA-1.5 13B.
\begin{center}
\begin{tcolorbox}[colback=gray!20,%gray background
                  colframe=black,
                  breakable,
                  title = {Template prompts of description generation}
                 ]
You are a helpful language and vision assistant. You are able to understand the visual content that the user provides and assist the user with a variety of tasks using natural language. I will give you an image and please describe this image. Please make sure that the generated descriptions should strictly adhere to the objects present in the image, without any nonexistent elements.\\
Below are the images to describe: [INSERT IMAGE HERE].
\end{tcolorbox}
\end{center}

In this example, the ‘[INSERT IMAGE HERE]’ works as the image placeholder which can be replaced by any image. Given the image shown in Fig.~\ref{img_exp}, the response of LLaVA-1.5 13B is:

\begin{figure}[t]
\centering
\includegraphics[width=0.3\linewidth]{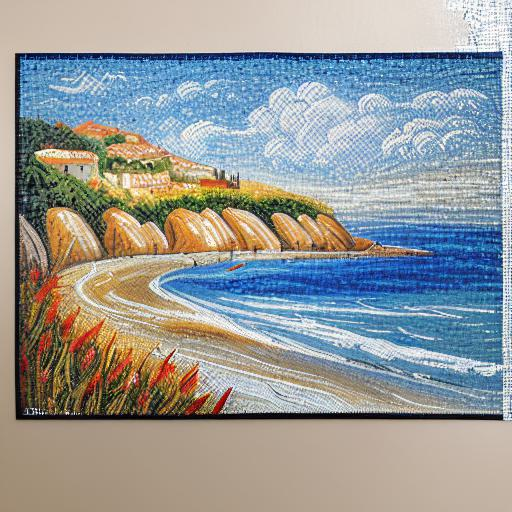}
\caption{Example image to be described.}
\label{img_exp}
\vspace{-8pt}
\end{figure}

\begin{center}
\begin{tcolorbox}[colback=gray!0,%gray background
                  colframe=black,
                  breakable,
                  title = {Examples of LLaVA response},
                  colbacktitle={white},
                  coltitle={black}
                 ]
The image features a colorful mosaic picture of a beach scene, with a sandy beach, a body of water, and a mountain in the background. The picture is displayed on a wall, likely in a room with a beach theme or a coastal view.
\end{tcolorbox}
\end{center}

\subsubsection{Evaluate editing by GPT-4V}
We ask GPT-4V to give quantitative scores on instruction-following consistency and content fidelity. The former represents how much the edited image faithfully follows the given instruction while the latter evaluates the consistency in subject, style, content, and image quality between the source and the edited image. Both scores are measured on a scale from 0 to 1. Detailed prompts are shown as:
\begin{center}
\begin{tcolorbox}[colback=gray!20,%gray background
                  colframe=black,
                  breakable,
                  title = {Template prompts of editing evaluation}
                 ]
                 
Hello ChatGPT, you are a helpful assistant.
For this task, I'll request you to don the hat of an art critic.
I'll present you with two artworks: ``Image 1'' and its derivative, ``Image 2'', which has been altered based on specific the instruction: [INSERT INSTRUCTION HERE].

Please assess these images on the following aspects:\\
1. Describe the modification changes in ``Image 2'' from ``Image 1'' considering subject, style, content, and image quality.

2. Evaluate if ``Image 2'' faithfully represents the given instruction. Provide a consistency score comparing the modification changes and the given instruction.

3. Quantify the resemblances between ``Image 1'' and ``Image 2'' on a scale from 0 to 1, and elucidate the reasons behind your scoring.
\\
For clarity, the evaluation tiers are:\\
Very poor: [0-0.2)\\
Poor: [0.2-0.4)\\
Fair: [0.4-0.6)\\
Good: [0.6-0.8)\\
Very good: [0.8-1.0]\\
Please give me the comprehensive assessments, evaluations, and scores. Finally, summarize answers point by point.\\
Below are the artworks in question: [INSERT IMAGE HERE].
\end{tcolorbox}
\end{center}

In this template, ``Image 1'' and ``Image 2'' denote the source and edited image, respectively. They will be placed in [INSERT IMAGE HERE] in order. The instruction used during the editing is denoted as [INSERT INSTRUCTION HERE]. 

\begin{figure}[htbp]
\centering
% \vspace{-0.4cm}    
    \subfloat[``Image 1'' ]{
        \includegraphics[width=0.2\linewidth]{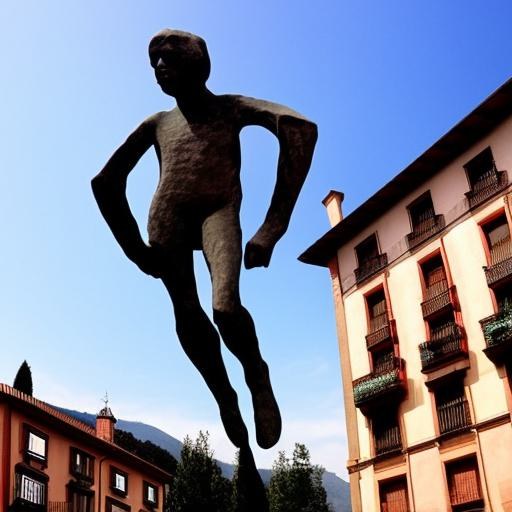}\label{image1}}
        \vspace{2pt}
    \subfloat[``Image 2'']{
        \includegraphics[width=0.2\linewidth]{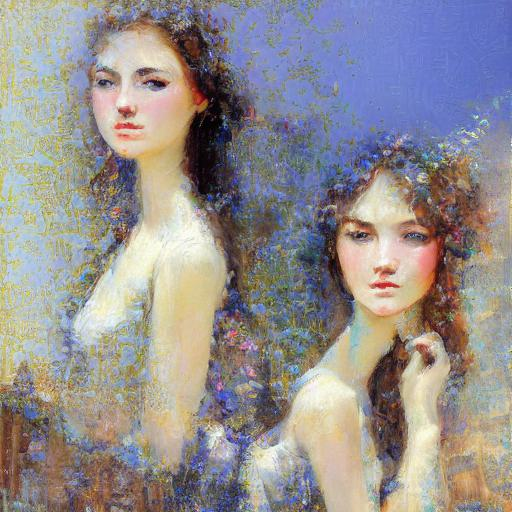}\label{image2}}
% \vspace{-0.2cm} 
\vspace{-5pt}
\caption{``source-edit'' pair that needed to be evaluated.}
\label{GPT4V-exp}
\vspace{-8pt}
\end{figure}

Given the image pair shown in Fig.~\ref{GPT4V-exp} and the instruction prompt \textit{``make the traveller a young woman''}, the evaluation output is:

\begin{center}
\begin{tcolorbox}[colback=gray!0,
                  colframe=black,
                  breakable,
                  title = {Examples of GPT-4V response},
                  colbacktitle={white},
                  coltitle={black}
                 ]
Certainly, let's assess these artworks.\\                 
1. Description of Modification Changes:

Subject: ``Image 1'' portrays a large sculpture of a figure, presumably a traveler, juxtaposed against urban architecture. ``Image 2'', in contrast, displays two young women, painted in a romanticized and delicate style.

Style: ``Image 1'' captures a realistic photographic style, emphasizing the magnitude and texture of the sculpture. ``Image 2'' adopts a painterly approach with soft brush strokes, pastel hues, and an impressionistic technique.

Content: While ``Image 1'' focuses on the sculpture and its surroundings, ``Image 2'' emphasizes the grace and beauty of the two young women, surrounded by floral elements.

Image Quality: Both images are clear and detailed in their respective mediums. ``Image 1'' excels in capturing real-world details, while ``Image 2" conveys emotion and texture through its brushwork.

2. Evaluation of Instruction Representation:

Given the instruction to ``make the traveler a young woman'', ``Image 2'' introduces young women but deviates greatly from the initial context and essence of ``Image 1''. The transformation is extensive, moving from a sculpture to a painted portrait.\\
Consistency Score: 0.2 (Very Poor)

3. Quantify Resemblances:

The two artworks are vastly distinct in both content and style.\\
Score: 0.1 (Very Poor)

Reasoning: Aside from both being visual artworks, the pieces share no evident similarities in terms of subject, style, or content.

Summary:

``Image 2'' makes a significant departure from ``Image 1'', transitioning from a photographic representation of a sculpture to an impressionistic painting of two young women.
While ``Image 2'' introduces young women, it does not faithfully capture the essence of ``making the traveller a young woman'', resulting in a consistency score of 0.2 (Very Poor).
The resemblance score between the two images is 0.1, underlining the marked differences in their subject, content, and style.
\end{tcolorbox}
\end{center}

\subsubsection{Generate instruction synonymous phrases}
We leverage GPT-3.5-Turbo to generate synonymous phrases for each original instruction prompt, to study the impact of instruction synonymous phrases. For each instruction, the model is asked to generate four synonymous phrases that will be further used to edit images. 
Here we give details of the prompt we used in our experiments.
\begin{center}
\begin{tcolorbox}[colback=gray!20,%gray background
                  colframe=black,
                  breakable,
                  title = {Template prompts of instruction synonym generation}
                 ]

Hello ChatGPT, you are a helpful assistant.\\
I will give you an instruction prompt that is used to edit an image: [INSERT INSTRUCTION HERE]\\
Please give me different instructions that satisfy:\\
1. have the similar meaning with the given prompt.\\
2. brief and concise.\\
3. use common vocabulary.\\
Please give me four different answers.
\end{tcolorbox}
\end{center}

Given the instruction \textit{``change the setting to a jungle''}, the output is:
\begin{center}
\begin{tcolorbox}[colback=gray!0,%gray background
                  colframe=black,
                  breakable,
                  title = {Examples of GPT-3.5 response},
                  colbacktitle={white},
                  coltitle={black}
                 ]
Certainly, here are four instructions with a similar meaning to ``change the setting to a jungle'' that are brief, use common vocabulary, and are easy to understand:

1. Replace the background with a jungle.\\
2. Transform the environment into a jungle.\\
3. Make the setting look like a jungle.\\
4. Swap the backdrop to a jungle scene.
\end{tcolorbox}
\end{center}

\subsection{Human evaluation}
We provide further details on the conducted user studies on image editing. Each participant is presented with twenty randomly selected ``source-edited'' image pairs with the protection of \method, along with corresponding instructions. Each participant is tasked with assessing editing performance, giving scores considering content fidelity, instruction following, and image quality. 

For the image fidelity study users have to answer the question: 
\begin{itemize}
    \item Does the edited image faithfully maintain the content that is presented in the source image?
    \item Does the editing faithfully follow the given instruction?
\end{itemize}
Users rate the images according to the rule similar as that of GPT-4V. In both cases the five answer options are: ``very poor'', ``poor'', ``fair'', ``good'' and ``very good''. For human, the rule of ``very poor'' with 0-0.2 is: The edited image does not follow the given directive and has significant inconsistencies. The content is significantly different. 
For ``very good'' with 0.8-1, the content of the image modification is completely consistent with the instructions and fully complies with human semantics. The edited image is a good representation of the original content.

To conduct our study, we randomly choose 50 participants from different ages and educational backgrounds. Each of them may be given different ``source-edited'' image pairs from two datasets, with the protection of \method. We calculate the percentage of each response and report the final results. 

\section{More Results\label{more_res}}
\subsection{Results on more image quality metrics}
We show image quality results of FID, PR, VIFp and FSIM metrics in Table~\ref{fid}. Results demonstrate that EditShield consistently outperforms PhotoGuard on image quality on various metrics.

\begin{table}[htbp]
\centering
% \vspace{-18pt}
\caption{Comparisons on image quality metrics over 200 images. We use Inception V3 as feature extractor for FID and VGG16 for PR. Both precision and recall are shown, separated by slashes. }
% \vspace{-8pt}
\resizebox{0.8\linewidth}{!}{
\begin{tabular}{ccccccc}
\toprule
\textbf{Dataset}                 & \textbf{Model}           & \textbf{Method} & FID$\uparrow$              & PR$\downarrow$                   & VIFp$\downarrow$           & FSIM$\downarrow$           \\\hline
\multirow{2}{*}{IPr2Pr} & \multirow{2}{*}{ip2p}    & Photoguard      & 139.380          & 0.898/0.913          & 0.034          & 0.123          \\
                                 &                          & EditShield      & \textbf{142.407} & \textbf{0.854/0.883} & \textbf{0.033} & \textbf{0.116} \\ \hline
\multirow{2}{*}{MagicBrush}      & \multirow{2}{*}{ip2p-mb} & Photoguard      & 152.957          & 0.990/0.971          & 0.174          & 0.465          \\
                                 &                          & EditShield      & \textbf{186.690} & \textbf{0.960/0.947} & \textbf{0.117} & \textbf{0.397}
\\ \bottomrule
\end{tabular}
}
\label{fid}
\end{table}

\subsection{Results on prompt-guided editing}
 EditShield can be applied to prompt-guided editing. We have shown some examples of EditShield in Null-text inversion~\cite{mokady2023null} in Fig~\ref{null}. We employ stable diffusion v1.4 using a DDIM sampler with number of diffusion steps T=50 and guidance scale=7.5. Results verify the generality of EditShield to prevent prompt-guided image editing.

 \begin{figure}[htbp]
% \vspace{-10pt}
\centering
    \setlength{\tabcolsep}{0pt} % Default value: 6pt
     % Default value: 1
\includegraphics[width=0.8\linewidth]{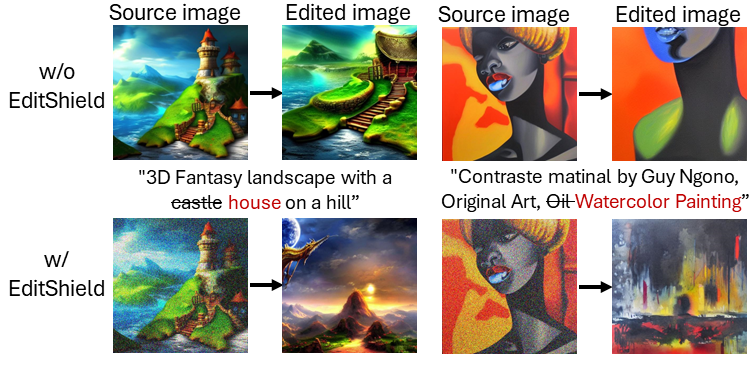}
% \vspace{-10pt}
    \caption{
    Qualitative protection results on Null-text inversion. 
    }
    \label{null}
    % \vspace{-20pt}
\end{figure}

\subsection{Results on newer models}
We apply EditShield to advanced instruction-based editing model MGIE~\cite{fu2023guiding} on IPr2Pr. Results in Fig.\ref{mgie} verifies the protection effectiveness.

\begin{figure}[htbp]
\vspace{-10pt}
\centering
\begin{minipage}[b]{0.54\linewidth}
    \centering
    \includegraphics[width=1\linewidth]{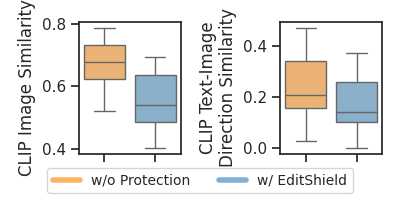}
    \vspace{-20pt}
    \caption{\scriptsize Quantitative results on MGIE.}
    \label{mgie}
\end{minipage}%
\hfill
\begin{minipage}[b]{0.44\linewidth}
    \centering
    \large
    \vspace{-8pt}
    
        \captionof{table}{Results on different distance metrics on ip2p. sim(img): CLIP image similarity; sim(dir): CLIP text-image direction similarity.  }
    \label{distance}
    \resizebox{1\linewidth}{!}{
        \begin{tabular}{ccc}
            \toprule
            \textbf{Metrics} & \textbf{$\Delta$ sim(img)} $\uparrow$ & \textbf{$\Delta$ sim(dir)} $\uparrow$ \\ \hline
            L-2 norm         & 0.012                      & 0.028                      \\
            MAE              & 0.016                      & 0.028                      \\
            MSE              & \textbf{0.023}             & \textbf{0.037}             \\ \bottomrule
        \end{tabular}
    }
    \vspace{-8pt}

\end{minipage}
\vspace{-10pt}
\end{figure}

\subsection{Ablation on distance metrics}
We show the median drop in two CLIP similarity metrics when using L-2 norm and mean absolute error (MAE) for distance metrics over 30 iterations on ip2p model. From Table~\ref{distance}, we observe that EditShield performs better with MSE than others.

\subsection{Ablation study on $\beta$\label{abaltion_beta}}
$\beta$ is the hyper-parameter to balance latent inconsistency loss and perceptual consistency loss. By default, we set $\beta$ to 0.2. Now we investigate the effect of it on our protection. We set $\beta$ to 0.1 and 0.3 and conduct experiments on IPr2Pr dataset. We calculate the median drop in two critical similarity metrics: CLIP image similarity and CLIP text-image direction similarity for measurement. Results are shown in Fig.~\ref{fig:beta}. 

With the increase of $\beta$, the protection effect slightly decreases. This is because less representation shift is caused by \method, resulting in degrading protection. By setting $\beta$ at 0.2, we can balance the protection effect and perturbation invisibility. 

\begin{figure*}[t]
\centering
% \vspace{-0.4cm}    
    \subfloat[Impact of $\beta$]{
        \includegraphics[width=0.4\linewidth]{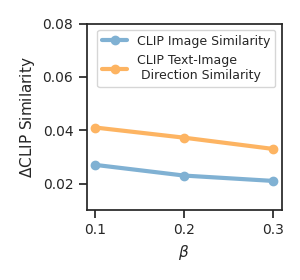}\label{fig:beta}}
        % \vspace{2pt}
    \subfloat[Impact of Set $D$]{
        \includegraphics[width=0.4\linewidth]{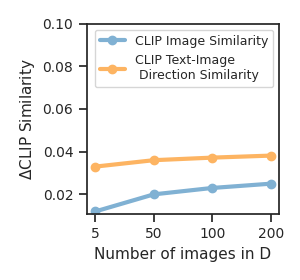}\label{setd}}
% \vspace{-0.2cm} 
% \vspace{-5pt}
\caption{Quantitative results on parameter sensitivity.}
\label{impact}
% \vspace{-16pt}
\end{figure*}

\subsection{Impact of sample size in Set $D$}
 We also study the impact of sample size in set $D$ on the protection performance. We show in Fig.~\ref{setd} the median drop of two similarity metrics obtained on 200 edited images, where the number of images in set $D$ varies from 5 to 200.

We use different numbers of images in Set $D$ to generate perturbations and add them to 2000 other images in IPr2Pr. From Fig.~\ref{setd}, protections generated from 100 examples show comparative effectiveness, indicating the generality of EditShield.
The decrease in the two similarity metrics is positively correlated with an increase in sample size, indicating that the effectiveness of protection perturbations improves with more samples used in the calculation. However, this improvement comes at the cost of increased computational resources. To balance the trade-off between protection and computational cost, we choose the ratio of sample size in $D$ to 0.25 in our default setting.

\subsection{Qualitative results on EOT}
We provide the comparison visualizations on the ablation of EOT in Fig.~\ref{ablation eot}. Results show that the integration of EOT does not substantially affect the visual quality.
\begin{figure}[htbp]

\centering
    \setlength{\tabcolsep}{0pt} % Default value: 6pt
     % Default value: 1
\includegraphics[width=0.75\linewidth]{figures/ablation eot.png}
\vspace{-8pt}
    \caption{
    Comparison and ablation on EOT from IPr2Pr dataset. 
    }
    \label{ablation eot}
\end{figure}

\subsection{More visualization results\label{vis}}
In addition to the discussion in the main text, we provide more qualitative examples in Fig.~\ref{sup_VIS1}. Each pair of rows displays the source and protected images with their respective edited versions. 

More examples of the robustness experiments, including different editing types and synonymous instruction phrases are shown in Fig.~\ref{sup_robustness}.

\begin{figure*}[t]
\centering
\includegraphics[width=0.9\linewidth]{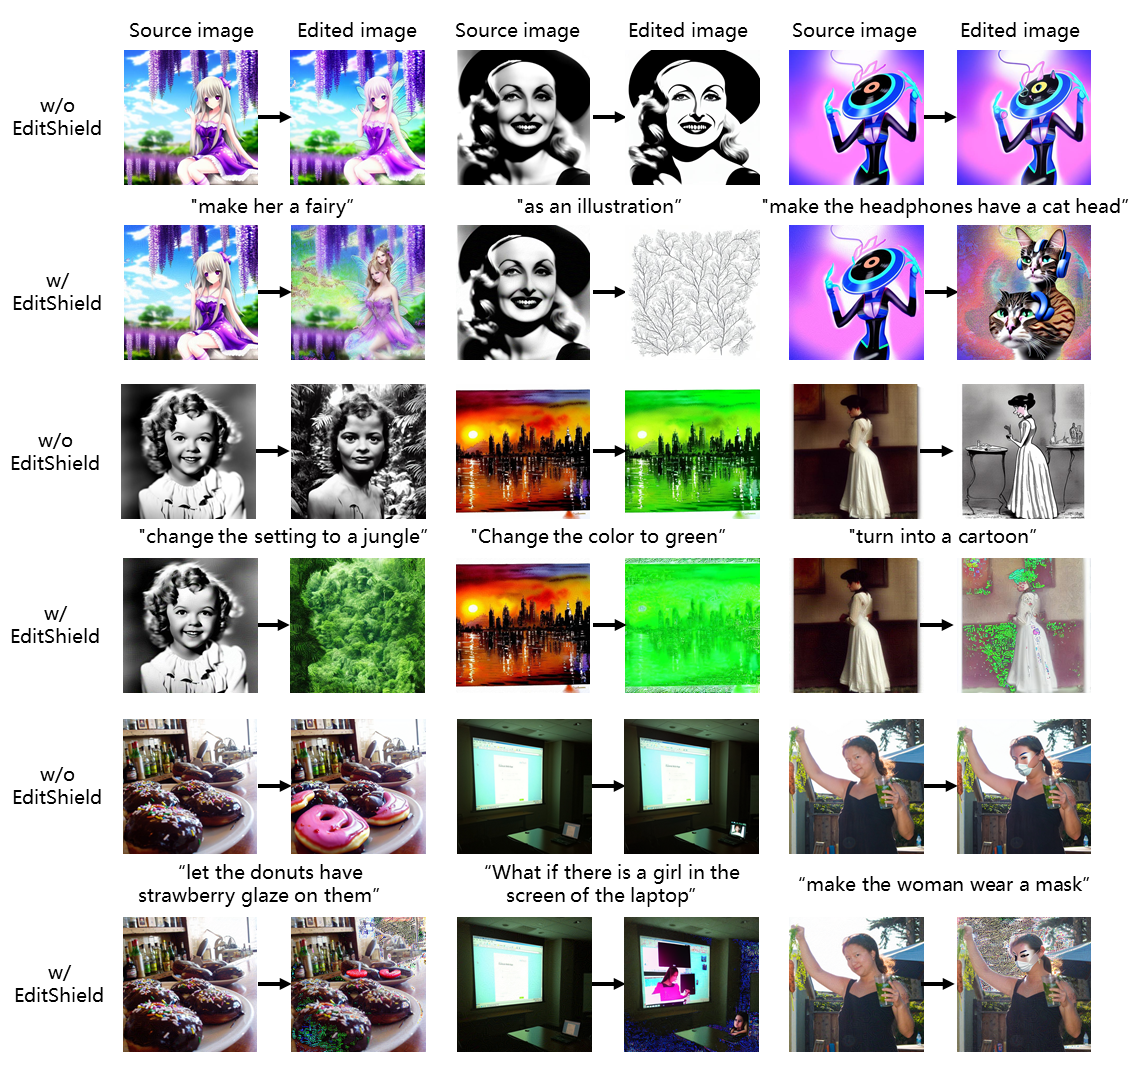}
\caption{Qualitative protection results. The source images and their corresponding instructions in uppermost four rows are from the training set of InstructPix2Pix while those in the last two rows are from MagicBrush.}
\label{sup_VIS1}
% \vspace{-8pt}
\end{figure*}

\begin{figure*}[t]
\centering
% \vspace{-0.4cm}    
    \subfloat[Editing types]{
        \includegraphics[width=0.46\linewidth]{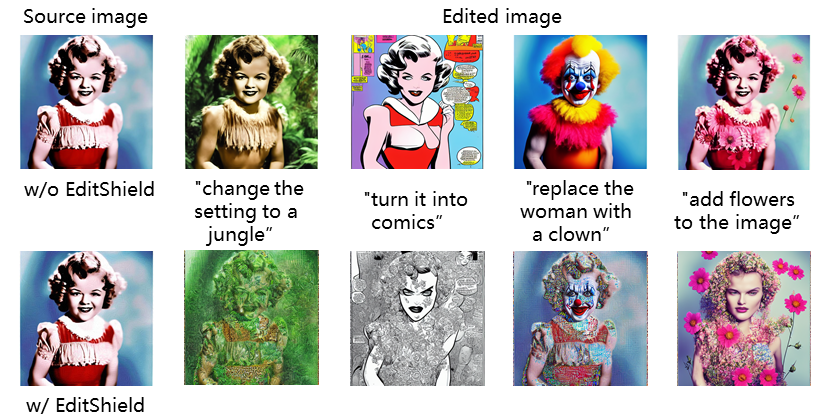}\label{type}}
        % \vspace{2pt}
    \subfloat[Synonymous instruction phrases]{
        \includegraphics[width=0.46\linewidth]{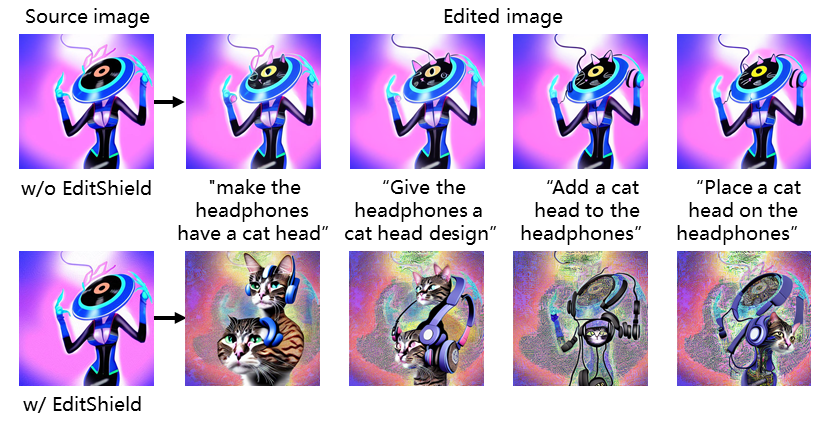}\label{variety}}
% \vspace{-0.2cm} 
% \vspace{-5pt}
\caption{Edited images with \method on different instructions.}
\label{sup_robustness}
% \vspace{-16pt}
\end{figure*}

% We observe that a relatively modest perturbation budget of 4/255 is sufficient for \method to significantly prevent the editing performance of instruction-guided image editing models, thereby leading to robust protection against unauthorized modifications. 

% \bibliographystyle{splncs04}
% \bibliography{egbib}

% \end{document}
